# Supplementary material for: Truncated Laplace and Gaussian mechanisms of RDP
Source: arXiv:2309.12647 source file (2023-09-22)
Supplement: Supplementary file 1 [file appendix.tex]

% \section{CDF of Gaussian}

% The probability that the Gaussian distribution $N(C,k)$ is smaller than $X = Z$ is denoted as follows, where K denotes the variance. For the second equation we used variable substitution, let $t = \frac{x-c}{\sqrt{2k}}$, so $x=\sqrt{2k}t+C$.

% \begin{align*}
% P(X<Z) &=\int_{-\infty}^{Z} \frac{1}{\sqrt{2 \pi k}} e^{-\frac{(x-C)^{2}}{2 k}} d x \\
% &=\int_{-\infty}^{\frac{Z-C}{\sqrt{2 k}}} \frac{1}{\sqrt{2 \pi k}} e^{-t^{2}}  d {(\sqrt{2k}t+C)} \\
% &=\int_{-\infty}^{\frac{Z-C}{\sqrt{2 k}}} \frac{1}{\sqrt{2 \pi k}} e^{-t^{2}} \sqrt{2 k} d t \\ 
% &=\int_{-\infty}^{\frac{Z-C}{\sqrt{2 k}}} \frac{1}{\sqrt{\pi}} e^{-t^{2}}  d t 
% \end{align*}

% Next, we let $k=(2C\sigma)^2$, $Z=\alpha C$, we can get:
% \begin{align*}
% P(X<Z) &=\int_{-\infty}^{\frac{Z-C}{\sqrt{2 k}}} \frac{1}{\sqrt{\pi}} e^{-t^{2}}  d t \\
% &=\int_{-\infty}^{\frac{\alpha C-C}{\sqrt{2 \cdot (2C\sigma)^2}}} \frac{1}{\sqrt{\pi}} e^{-t^{2}}  d t \\
% &=\int_{-\infty}^{\frac{\alpha-1 }{2\sqrt{2} \sigma}} \frac{1}{\sqrt{\pi}} e^{-t^{2}}  d t 
% \end{align*}

\section{Network Model}
\label{sec:appendix model}
We use the network architectures of all experiment are the same as previous work \cite{FlorianTramr2020DifferentiallyPL,Wei_Bao_Xiao_Yang_2022,NicolasPapernot2020TemperedSA}.
\vspace{5mm}
\begin{table}[h]
\centering
\caption{MNIST and FashionMNIST model architecture}
\begin{tabular}{@{}ll@{}}
\toprule
Layer & \text {Parameters} \\
\midrule
Convolution & \text {16 filters of 8$\times$8, stride 2,padding 2} \\
Max-Pooling & \text {2$\times$2, stride 1 } \\
Convolution & \text {32 filters of 4$\times$4, stride 2, padding 0} \\
Max-Pooling & \text {2$\times$2, stride 1 } \\
Fully connected & \text {32 units} \\
Fully connected & \text {10 units} \\
\bottomrule
\end{tabular}
\label{table:MNIST and FMNIST model}

\end{table}

\begin{table}[h]
\centering
\caption{ CIFAR10 model architecture}
\begin{tabular}{@{}ll@{}}
\toprule
Layer & \text {Parameters} \\
\midrule
Convolution$\times$2 & \text {32 filters of 3$\times$3, stride 1, padding 1} \\
Max-Pooling & \text {2$\times$2, stride 2 } \\
Convolution$\times$2 & \text {64 filters of 3$\times$3, stride 1, padding 1} \\
Max-Pooling & \text {2$\times$2, stride 2 } \\
Convolution$\times$2 & \text {128 filters of 3$\times$3, stride 1, padding 1} \\
Max-Pooling & \text {2$\times$2, stride 2 } \\
Fully connected & \text {128 units} \\
Fully connected & \text {10 units} \\
\bottomrule
\end{tabular}
\label{table:CIFAR-10 model}
\end{table}

\begin{table}[h]
    \caption{IMDb model architecture.}
    \centering
    \begin{tabular}{l|l}
        \toprule
        Layer & Parameters \\
        \midrule
        Embedding & 100 units \\
        Fully connected & 32 units \\
        Bidirectional LSTM & 32 units \\
        Fully connected & 16 units \\
        Fully connected & 2 units \\
        \bottomrule
    \end{tabular}
    \label{table:IMDb model}
\end{table}

\section{Parameter settings}
\label{sec:parameter settings}

\vspace{5mm}
\begin{table}[h]
\centering
\caption{The setting of hyperparameters in MNIST}
\begin{tabular}{lcccc}
\toprule
Parameter & \text {$\epsilon=1$} & \text{$\epsilon=2$} & \text{$\epsilon=3$} & \text{$\epsilon=4$} \\
\midrule
Learning rate $\eta$ & 2.0 & 2.0 & 2.0 & 2.0 \\
Batch size $B$ & 1024 & 1024 & 1024 & 1024 \\
Clipping norm $C$ & 0.1 & 0.1 & 0.1 & 0.1 \\
Noise multiplier $\sigma$ & 2.0 & 1.5 & 1.35 & 1.35 \\
\bottomrule
\end{tabular}
\label{table:parameter settings in MNIST}
\vspace{5mm}
\end{table}

\begin{table}[h]
\centering
\caption{The setting of hyperparameters in FMNIST}
\begin{tabular}{lcccc}
\toprule
Parameter & \text {$\epsilon=1$} & \text{$\epsilon=2$} & \text{$\epsilon=3$} & \text{$\epsilon=4$} \\
\midrule
Learning rate $\eta$ & 4.0 & 4.0 & 4.0 & 4.0 \\
Batch size $B$ & 2048 & 2048 & 2048 & 2048 \\
Clipping norm $C$ & 0.1 & 0.1 & 0.1 & 0.1 \\
Noise multiplier $\sigma$ & 4.0 & 2.15 & 2.15 & 2.15 \\
\bottomrule
\end{tabular}
\label{table:parameter settings in FMNIST}
\vspace{5mm}
\end{table}

\begin{table}[h]
\centering
\caption{The setting of hyperparameters in CIFAR-10}
\begin{tabular}{lcccc}
\toprule
Parameter & \text {$\epsilon=1$} & \text{$\epsilon=2$} & \text{$\epsilon=3$} & \text{$\epsilon=4$} \\
\midrule
Learning rate $\eta$ & 4.0 & 4.0 & 4.0 & 4.0 \\
Batch size $B$ & 8192 & 8192 & 8192 & 8192 \\
Clipping norm $C$ & 0.1 & 0.1 & 0.1 & 0.1 \\
Noise multiplier $\sigma$ & 10.0 & 9.0 & 5.67 & 5.67 \\
\bottomrule
\end{tabular}
\label{table:parameter settings in CIFAR10}
\vspace{5mm}
\end{table}

\begin{table}[h]
\centering
\caption{The setting of hyperparameters in IMDB}
\begin{tabular}{lcccc}
\toprule
Parameter & \text {$\epsilon=1$} & \text{$\epsilon=2$} & \text{$\epsilon=3$} & \text{$\epsilon=4$} \\
\midrule
Learning rate $\eta$ & 0.02 & 0.02 & 0.02 & 0.02 \\
Train batch size $B$ & 1024 & 1024 & 1024 & 1024 \\
Train clipping norm $C$ & 0.1 & 0.1 & 0.1 & 0.1 \\
Train noise multiplier $\sigma$ & 2.0 & 1.8 & 1.35 & 1.23 \\
\bottomrule
\end{tabular}
\label{table:parameter settings in IMDB}
\end{table}

\section{Proof of Gaussian Mechanism with Selective Release}
\label{sec:Proof of Gaussian mechanism with selective publish}
\begin{align}
\begin{split} 
\begin{aligned}
D_{\alpha}( & f(x ; 0, \mu\sigma, a, b )||f(x ; \mu, \mu\sigma, a, b)) \\
= & \frac{1}{\alpha-1} \cdot \frac{(\Phi(\frac{b-u}{\mu\sigma })-\Phi(\frac{a-u}{\mu\sigma } ))^\alpha  }{(\Phi(\frac{b}{\mu\sigma })-\Phi(\frac{a}{\mu\sigma }))^{\alpha-1}} \cdot  \log \int_{a}^{b} \frac{1}{\mu\sigma \sqrt{2 \pi}} \exp \left(-\alpha x^{2} /\left(2 \mu^2\sigma^2\right)\right) \\
& \cdot \exp \left(-(1-\alpha)(x-\mu)^{2} /\left(2 \mu^2\sigma^2\right)\right) \mathrm{d} x \\
= & \frac{1}{\alpha-1}\cdot \frac{(\Phi(\frac{b-u}{\mu\sigma })-\Phi(\frac{a-u}{\mu\sigma } ))^\alpha  }{(\Phi(\frac{b}{\mu\sigma })-\Phi(\frac{a}{\mu\sigma }))^{\alpha-1}} \cdot \log \frac{1}{\mu\sigma \sqrt{2 \pi}} \int_{a}^{b} \exp \left[\left(-x^{2}+\right.\right. \\
& \left.\left.2(1-\alpha) \mu x-(1-\alpha) \mu^{2}\right) /\left(2 \mu^2\sigma^2\right)\right] \mathrm{d} x \\
= & \frac{1}{\alpha-1} \cdot \frac{(\Phi(\frac{b-u}{\mu\sigma })-\Phi(\frac{a-u}{\mu\sigma } ))^\alpha  }{(\Phi(\frac{b}{\mu\sigma })-\Phi(\frac{a}{\mu\sigma }))^{\alpha-1}} \cdot  \log \frac{1}{\sqrt{\pi}} \int_{a}^{b} exp(\frac{\alpha(\alpha -1)}{2\sigma^2 })  \\
& \cdot exp(-(\frac{x-(1-\alpha)}{\sqrt[]{2}\sigma })^2 )\mathrm{d}(\frac{x-(1-\alpha)}{\sqrt[]{2}\sigma })\\
= & \frac{1}{\alpha-1} \cdot \frac{(\Phi(\frac{b-\mu}{\mu\sigma })-\Phi(\frac{a-\mu}{\mu\sigma } ))^\alpha  }{(\Phi(\frac{b}{\mu\sigma })-\Phi(\frac{a}{\mu\sigma }))^{\alpha-1}} \cdot  (\frac{a(a-1)}{2\sigma ^2} \\
& + \log [{\Phi(\frac{b-(1-\alpha)}{\sqrt{2}\sigma})-\Phi(\frac{a-(1-\alpha)}{\sqrt{2}\sigma})}]/\sqrt{2} )\\
= & \frac{(\Phi(\frac{b-\mu}{\mu\sigma })-\Phi(\frac{a-\mu}{\mu\sigma } ))^\alpha  }{(\Phi(\frac{b}{\mu\sigma })-\Phi(\frac{a}{\mu\sigma }))^{\alpha-1}} \cdot  (\frac{\alpha }{2 \sigma^2} +\log[(\Phi(\frac{b-(1-\alpha)}{\sqrt{2}\sigma})\\
& -\Phi(\frac{a-(1-\alpha)}{\sqrt{2}\sigma}))/\sqrt{2}(\alpha -1)] ,\\
& \textrm{where} \; \Phi(x)=\frac{1}{\sqrt{2 \pi}} \int_{-\infty}^{x} e^{-\frac{t^{2}}{\sqrt{2}}} dt \nonumber.
\end{aligned}
\end{split}
\end{align}
%%% Local Variables:
%%% mode: latex
%%% TeX-master: "main"
%%% End:
